# Supplementary material for: A Unified Analysis of Variational Inequality Methods: Variance Reduction, Sampling, Quantization and Coordinate Descent
Source: arXiv:2201.12206 source file (2022-02-03)
Supplement: Supplementary file 1 [file appendix.tex]

\section{Приложение}
\subsection{Вспомогательные результаты}

В данном подразделе привед\ev{ё}м некоторые леммы из других работ, на которые мы будем ссылаться в доказательствах. Также привед\ev{ё}м доказательства утверждений о свойствах двойственной функции, которые используются \ev{при} доказательстве основных теорем. 

\begin{Lem}[Лемма~2 из \cite{jin2019short}]\label{lem:jin_lemma_2}
    Для случайного вектора  $\xi \, \in  \, \RR^n$ следующие утверждения эквивалентны с точностью до константного множителя у  $\sigma$\ev{:}
    \begin{enumerate}
        \item Хвосты: $\PP\left\{\|\xi\|_2 \ge \gamma\right\} \le 2 \exp\left(-\frac{\gamma^2}{2\sigma^2}\right)$ $\forall \gamma \ge 0$.
        \item Моменты: $\left(\EE\left[\xi^p\right]\right)^{\frac{1}{p}} \le \sigma\sqrt{p}$ для любого положительного целого $p$.
        \item  Предположение легких хвостов: $\EE\left[\exp\left(\frac{\|\xi\|_2^2}{\sigma^2}\right)\right] \le \exp(1)$.
    \end{enumerate}
\end{Lem}

\begin{Lem}[Следствие~8 из \cite{jin2019short}]\label{lem:jin_corollary}
    Пусть $\{\xi^k\}_{k = 1}^N$~\ev{---} последовательность случайных векторов из $\RR^n$\ev{,} таки\ev{x,} что для  $k=1, \, \ldots, \, N$ и для любых $\gamma \ge 0$
    \begin{equation*}
        \EE\left[\xi^k\mid \xi^1, \, \ldots, \, \xi^{k-1}\right] = 0,\quad \EE\left[\|\xi^k\|_2 \ge \gamma \mid \xi^1, \, \ldots, \, \xi^{k-1}\right] \, \le \, \exp\left(-\frac{\gamma^2}{2\sigma_k^2}\right)\quad \text{почти наверное,}
    \end{equation*}
    где $\sigma_k^2$ принадлежит $\sigma(\xi^1, \, \ldots, \, \xi^{k-1})$ для всех $k=1, \, \ldots, \, N$. Пусть $S_N = \sum\limits_{k=1}^N\xi^k$. Тогда существует константа $C_1$\ev{,} такая что для любых фиксированных $\delta > 0$ и $B > b > 0$ с вероятностью $1 - \delta$ \ev{выполняется}:
    \begin{equation*}
        \text{либо } \sum\limits_{k=1}^N\sigma_k^2 \ge B\ev{,} \quad \text{либо} \quad \|S_N\|_2 \le C_1\sqrt{\max\left\{\sum\limits_{k=1}^N\sigma_k^2, \, b\right\}\left(\ln\frac{2n}{\delta} + \ln\ln\frac{B}{b}\right)}.
    \end{equation*}
\end{Lem}

\begin{Lem}[Следствие из теоремы~2.1, случай  (ii) из \cite{JudNem}]\label{lem:jud_nem_large_dev}
    Пусть $\{\xi^k\}_{k = 1}^N$~\ev{---} последовательность случайных векторов из $\RR^n$ \ev{удовлетворяет условию}% такая что
    \begin{equation*}
        \EE\left[\xi^k\mid \xi^1, \, \ldots, \, \xi^{k-1}\right] = 0 \text{ почти наверное,}\quad k=1, \, \ldots, \, N
    \end{equation*}
    и пусть $S_N = \sum\limits_{k=1}^N\xi^k$. Пусть последовательность $\{\xi^k\}_{k = 1}^N$ удовлетвояет ``light-tail''\ev{-}условию:
    \begin{equation*}
        \EE\left[\exp\left(\frac{\|\xi^k\|_2^2}{\sigma_k^2}\right)\mid \xi^1, \, \ldots, \, \xi^{k-1}\right] \, \le \, \exp(1) \text{ почти наверное,}\quad k = 1, \, \ldots, \, N,
    \end{equation*}
    где $\sigma_1,\ldots,\sigma_N$~\ev{---} положительные числа. Тогда для всех $\gamma \, \ge \, 0$ \ev{выполняется}
    \begin{equation}
        \PP\left\{\|S_N\| \ge \left(\sqrt{2} + \sqrt{2\gamma}\right)\sqrt{\sum\limits_{k=1}^N\sigma_k^2}\right\} \le \exp\left(-\frac{\gamma^2}{3}\right).
    \end{equation}
\end{Lem}

\textbf{Доказательство утверждения \ref{2_cor_sopr}}

Представим двойственную функцию в следующем виде

\begin{eqnarray*}
    \varphi(\boldsymbol{\lambda})= \sum_{k = 1}^{n}  \left \{ u_k(x_k(\boldsymbol{\lambda})) - \langle\boldsymbol{\lambda}, \, \mathbf{C}_k \rangle x_k(\boldsymbol{\lambda}) + \dfrac{1}{n}\langle \boldsymbol{\lambda}, \, \mathbf{b} \rangle \right \} =\sum_{k = 1}^{n} \varphi_k(\boldsymbol{\lambda}),
\end{eqnarray*}
при этом из утверждения \ref{2_cor_dem} получаем, что
\begin{eqnarray*}
    \nabla \varphi(\boldsymbol{\lambda}) = \sum_{k = 1}^{n} \nabla \varphi_k(\boldsymbol{\lambda}) = \sum_{k = 1}^{n} \left( \frac{1}{n} \mathbf{b} -\mathbf{C}_k x_k(\boldsymbol{\lambda})  \right).
\end{eqnarray*}
Определим 
\begin{eqnarray*}
    x_k(\boldsymbol{\lambda}\ev{^1})  =  \argmax_{x_k \, \in \, \RR_+} \left \{
    u_k(x_k) - x_k \langle \boldsymbol{\lambda}\ev{^1}, \mathbf{C}_k \rangle
    \right \}, \quad x_k(\boldsymbol{\lambda}\ev{^2})  =  \argmax_{x_k \, \in \, \RR_+} \left \{
    u_k(x_k) - x_k \langle \boldsymbol{\lambda}\ev{^2}, \mathbf{C}_k \rangle
    \right \}.
\end{eqnarray*}
Запишем необходимые условия максимума первого порядка \begin{eqnarray*}
    & \left \langle \nabla u_k(x_k(\boldsymbol{\lambda}\ev{^1})) - \langle \boldsymbol{\lambda}\ev{^1}, \, \mathbf{C}_k \rangle, \, x_k(\boldsymbol{\lambda}\ev{^1}) - x_k(\boldsymbol{\lambda}\ev{^2}) \right \rangle \geq 0 
    , \\
    &\left \langle \nabla u_k(x_k(\boldsymbol{\lambda}\ev{^2})) - \langle \boldsymbol{\lambda}\ev{^2}, \, \mathbf{C}_k \rangle, \, x_k(\boldsymbol{\lambda}\ev{^2}) - x_k(\boldsymbol{\lambda}\ev{^1}) \right \rangle \geq 0.
\end{eqnarray*}
Складывая эти неравенства, получаем 
\begin{eqnarray*}
\left    \langle \nabla u_k(x_k(\boldsymbol{\lambda}\ev{^2})) - \nabla u_k(x_k(\boldsymbol{\lambda}\ev{^1})), \, x_k(\boldsymbol{\lambda}\ev{^1}) -  x_k(\boldsymbol{\lambda}\ev{^2}) \right \rangle \leq 
    \left   \langle \langle \boldsymbol{\lambda}\ev{^2}, \, \mathbf{C}_k \rangle  - \langle \boldsymbol{\lambda}\ev{^1}, \, \mathbf{C}_k \rangle,  \, x_k(\boldsymbol{\lambda}\ev{^1}) -  x_k (\boldsymbol{\lambda}\ev{^2}) \right \rangle.
\end{eqnarray*}
\ev{В силу} сильной вогнутости $u_k(x_k)$ \ev{для любых $x_k^1$ и
$x_k^2$, $k = 1, \, \ldots, \, n$, выполняется}% получаем следующее соотношение 
\begin{eqnarray*}
    \langle \nabla u_k(x_k^2) - \nabla u_k(x_k^1), \, x_k^1 -  x_k^2 \rangle \geq \mu ||x_k^1 - x_k^2||^2_2.
\end{eqnarray*}
Отсюда получаем, что 
\begin{eqnarray*}
    \mu ||x_k(\boldsymbol{\lambda}\ev{^1}) - x_k(\boldsymbol{\lambda}\ev{^2})||^2_2 &\leq &
       \langle \langle \boldsymbol{\lambda}\ev{^2}, \, \mathbf{C}_k \rangle  - \langle \boldsymbol{\lambda}\ev{^1}, \, \mathbf{C}_k \rangle,  \, x_k(\boldsymbol{\lambda}\ev{^1}) -  x_k(\boldsymbol{\lambda}\ev{^2}) \rangle \\ &\leq& ||\mathbf{C}_k ||_2 \cdot ||\boldsymbol{\lambda}\ev{^1} - \boldsymbol{\lambda}\ev{^2}||_2 \cdot ||x_k(\boldsymbol{\lambda}\ev{^1}) - x_k(\boldsymbol{\lambda}\ev{^2})||_2.
\end{eqnarray*}
Тогда можно получить следующую оценку \ev{для всех $\nabla \varphi_k$}%на $k$-ую компоненту градиента 
\begin{eqnarray*}
    ||\nabla \varphi_k(\boldsymbol{\lambda}\ev{^1})-\nabla \varphi_k(\boldsymbol{\lambda}\ev{^2})||_2 \leq ||\mathbf{C}_k ||_2 \cdot ||x_k(\boldsymbol{\lambda}\ev{^1}) - x_k(\boldsymbol{\lambda}\ev{^2})||_2 \leq \frac{1}{\mu}
 ||\mathbf{C}_k ||^2_2 \cdot ||\boldsymbol{\lambda}\ev{^1} - \boldsymbol{\lambda}\ev{^2}||_2.
\end{eqnarray*}
\ev{Для матрицы $C$ c учётом её структуры верна оценка }%Учитывая структуру матрицы $C$, получаем, что 
$||\mathbf{C}_k ||_2 \leq m$. Тогда %получаем следующую оценку 
для градиента двойственной функции
\begin{eqnarray*}
    ||\nabla \varphi(\boldsymbol{\lambda}\ev{^1})-\nabla \varphi(\boldsymbol{\lambda}\ev{^2})||_2 \leq \sum_{k = 1}^{n}
    ||\nabla \varphi_k(\boldsymbol{\lambda}\ev{^1})-\nabla \varphi_k(\boldsymbol{\lambda}\ev{^2})||_2 \leq \frac{m^2n}{\mu} ||\boldsymbol{\lambda}\ev{^1} - \boldsymbol{\lambda}\ev{^2}||_2.
 \quad   \blacksquare
\end{eqnarray*}

\subsection{Доказательство леммы~\ref{lem_est_1}}

Для доказательства леммы~\ref{lem_est_1} сначала сформулируем и докажем одну техническую лемму. 

Обозначим $\evv{d_L}%\psi_0
(\boldsymbol{\lambda}) = 
\frac{L}{2} \| \boldsymbol{\lambda} - \boldsymbol{\lambda^0} \|_2^2$ и
рассмотрим последовательности
%$$
%\psi_i(\lambda) = \frac{L}{2} \| \lambda - \lambda_0 \|_2^2 +			\sum\limits_{j = 0}^i \alpha_j \left [ 
%\varphi(\lambda_j) + 
%			\nabla \varphi (\lambda_j) (\lambda - \lambda_j)
		%	\right ] 
%$$
%и
$$
l_t(\boldsymbol{\lambda}) = \sum\limits_{j = 0}^t \alpha_j \left [ 
\varphi(\boldsymbol{\lambda}^j) + \langle
			\nabla \varphi (\boldsymbol{\lambda}^j), \boldsymbol{\lambda} - \boldsymbol{\lambda}^j\rangle 
			\right ] 
$$
и
$$
\psi_{\evv{t}%t+1
}(\boldsymbol{\lambda}) = l_t(\boldsymbol{\lambda}) + \evv{d_L}%\psi_0
(\boldsymbol{\lambda}), \evv{t = 0, \, 1, \, \ldots}
$$
где $\{ \boldsymbol{\lambda}^j \}_{j \, \ge \, 0}$~--- последовательность точек, генерируемых алгоритмом~\ref{alg_fgm}.

%------------Лемма 9
\begin{Lem}\label{lem_fgm_pd}
После $N$ шагов алгоритма~\ref{alg_fgm}
выполняется следующее неравенство:
\begin{equation}
\label{eq_lem1}
A_N \varphi(\mathbf{y}^N) \, \le \, \min_{\boldsymbol{\lambda} \, \in \, \RR_{+}^m}
\psi_N (\boldsymbol{\lambda}) = \psi_N(\mathbf{z}^N).
\end{equation}
\end{Lem}

\textbf{Доказательство леммы \ref{lem_fgm_pd}}

Докажем по индукции, что \eqref{eq_lem1} верно. 
При $t = 0$ неравенство~\eqref{eq_lem1} выполняется.
\evv{Действительно, 
\begin{eqnarray}
\psi_0 & = & \min_{\boldsymbol{\lambda} \, \in \, \RR_{+}^m}
\left \{
\alpha_0 \left [ 
\varphi(\boldsymbol{\lambda}^0) + \langle
			\nabla \varphi (\boldsymbol{\lambda}^0), \boldsymbol{\lambda} - \boldsymbol{\lambda}^0\rangle 
			\right ] +
			\frac{L}{2} \| \boldsymbol{\lambda} - \boldsymbol{\lambda^0} \|_2^2
\right \}
 \notag \\
& \overset{\circledOne}{\ge} &
\alpha_0
\min_{\boldsymbol{\lambda} \, \in \, \RR_{+}^m}
\left \{ 
\varphi(\boldsymbol{\lambda}^0) + \langle
			\nabla \varphi (\boldsymbol{\lambda}^0), \boldsymbol{\lambda} - \boldsymbol{\lambda}^0\rangle 
			 +
			\frac{L}{2} \| \boldsymbol{\lambda} - \boldsymbol{\lambda^0} \|_2^2
\right \} 
\, \overset{\circledTwo}{\ge} \, \alpha_0 \varphi(y_0),
\nonumber
\end{eqnarray}
где
$\circledOne$ выполняется, так как 
$\alpha_0 = 1/2 \, \le \, 1$,
а $\circledTwo$~--- в силу того, что функция
$\varphi(\boldsymbol{\lambda})$ имеет липшицев
градиент (см. Утверждение~\ref{2_cor_sopr}
и \cite[Лемма 1.2.3]{nesterov_book2018}).
Итак, $A_0 \varphi(\mathbf{y}^0) = \frac{1}{2}
\varphi(\mathbf{y}^0) \, \le \, \psi_0$.
}
%-----------------------------------

Пусть \eqref{eq_lem1} верно при $t$:
\begin{equation}
\label{eq_ind_pred}
A_t \varphi(\mathbf{y}^t) \, \le \, \psi_t(\mathbf{z}^t).
\end{equation}
Докажем, что \eqref{eq_lem1} верно при $t+1$.
Действительно,
\begin{eqnarray}
\label{eq_last_in_lem1}
\psi_{t+1}(\mathbf{z}^{t+1}) & =& \min_{\boldsymbol{\lambda} \, \in \, \RR_{+}^m}
\left \{
\psi_t(\boldsymbol{\lambda}) + \alpha_{t+1}
\left [ 
\varphi(\boldsymbol{\lambda}^{t+1}) + 
			\langle	\nabla \varphi (\boldsymbol{\lambda}^{t+1}), \boldsymbol{\lambda} - \boldsymbol{\lambda}^{t+1}\rangle 
			\right ] 
\right \} \notag \\
&
\overset{\circledOne}{\ge}& \, 
\min_{\boldsymbol{\lambda} \, \in \, \RR_{+}^m}
\left \{
\psi_t(\mathbf{z}^t) + \frac{L}{2} \| \boldsymbol{\lambda} - \mathbf{z}^t \|_2^2 +
\alpha_{t+1}
\left [ 
\varphi(\boldsymbol{\lambda}^{t+1}) + 
		\langle	\nabla \varphi (\boldsymbol{\lambda}^{t+1}), \boldsymbol{\lambda} - \boldsymbol{\lambda}^{t+1}\rangle 
			\right ] 
\right \} \notag  \\
&
\overset{\circledTwo}{\ge}& \,
\min_{\boldsymbol{\lambda} \, \in \, \RR_{+}^m}
\left \{
A_t \varphi(\mathbf{y}^t) + \frac{L}{2} \| \boldsymbol{\lambda} - \mathbf{z}^t \|_2^2 +
\alpha_{t+1}
\left [ 
\varphi(\boldsymbol{\lambda}^{t+1}) + 
		\langle	\nabla \varphi (\boldsymbol{\lambda}^{t+1}), \boldsymbol{\lambda} - \boldsymbol{\lambda}^{t+1}\rangle 
			\right ] 
\right \} \notag 
\\ &
\overset{\circledThree}{\ge} &\,
\min_{\boldsymbol{\lambda} \, \in \, \RR_{+}^m}
\Bigg \{
A_t \left ( \varphi(\boldsymbol{\lambda}^{t+1}) + \langle	\nabla \varphi (\boldsymbol{\lambda}^{t+1}), \boldsymbol{\lambda} - \boldsymbol{\lambda}^{t+1}\rangle  \right ) +
\frac{L}{2} \| \boldsymbol{\lambda} - \mathbf{z}^t \|_2^2 \notag  \\ & +&
\alpha_{t+1}
\left [ 
\varphi(\boldsymbol{\lambda}^{t+1}) 
 + \langle	\nabla \varphi (\boldsymbol{\lambda}^{t+1}), \boldsymbol{\lambda} - \boldsymbol{\lambda}^{t+1}\rangle 
			\right ] 
\Bigg \}.
\end{eqnarray}
где $\circledOne$ выполняется в силу \evv{сильной выпуклости прокс-функции
$\frac{1}{2} \| \boldsymbol{\lambda} - \boldsymbol{\lambda^0} \|_2^2$
и свойств экстремума в точке $\mathbf{z}^t$},
$\circledTwo$ следует из~\eqref{eq_ind_pred},
$\circledThree$~--- в силу выпуклости функции $\varphi(\boldsymbol{\lambda})$.

Так как между коэффициентами $A_t$ и $\alpha_t$ БГМ есть следующая зависимость:
$A_{\evv{t+1}} = \sum\limits_{j=0}^{\evv{t+1}} \alpha_{\evv{j}} = A_t + \alpha_{t+1}$ и $\tau_t = \alpha_{t+1} / A_{t+1}$, соотношение $\boldsymbol{\lambda}^{t + 1} = \tau_t \mathbf{z}^t + (1 - \tau_t) \mathbf{y}^t$ из алгоритма~\ref{alg_fgm} можно переписать
так:
$$
A_{t+1} \boldsymbol{\lambda}^{t+1} = \alpha_{t+1} \mathbf{z}^t + A_t \mathbf{y}^t.
$$
Используя последние соотношения, можно сделать следующие
преобразования:
\begin{eqnarray*}
& A_t  \langle  \nabla \varphi (\boldsymbol{\lambda}^{t+1}), \mathbf{y}^t - \boldsymbol{\lambda}^{t+1} \rangle  + \alpha_{t+1} \langle \nabla \varphi(\boldsymbol{\lambda}^{t+1}) , \boldsymbol{\lambda} - \boldsymbol{\lambda}^{t+1} \rangle  \evv{ =}\\ &
\evv{=} - A_{t+1} \langle \nabla \varphi(\boldsymbol{\lambda}^{\evv{t+1}}), \boldsymbol{\lambda}^{t+1} \rangle  + \alpha_{t+1} \langle \nabla \varphi(\boldsymbol{\lambda}^{t+1}), \,
\boldsymbol{\lambda} \rangle + A_t \langle \nabla \varphi(\boldsymbol{\lambda}^{t+1}), \, \mathbf{y}^t \rangle \evv{ =}\\ 
&  = 
\alpha_{\evv{t}+1} 
\evv{\langle}
\nabla \varphi(\boldsymbol{\lambda}^{\evv{t+1}}), \, \boldsymbol{\lambda} - \mathbf{z}^{\evv{t}}
\evv{\rangle}.
\end{eqnarray*}
Тогда 
$$
A_t \left ( \varphi(\boldsymbol{\lambda}^{t+1}) + \langle \nabla \varphi(\boldsymbol{\lambda}^{t+1}),
\mathbf{y}^t - \boldsymbol{\lambda}^{t+1} \rangle \right ) +
\frac{L}{2} \| \boldsymbol{\lambda} - \mathbf{z}^t \|_2^2 +
\alpha_{t+1}
\left [ 
\varphi(\boldsymbol{\lambda}^{t+1}) + 
		\evv{\langle}	\nabla \varphi (\boldsymbol{\lambda}^{t+1}), \, \boldsymbol{\lambda} - \boldsymbol{\lambda}^{t+1}
		\evv{\rangle}
			\right ] =
$$
\begin{equation}
\label{eq_last_eq_lem1}
= A_{t+1} \varphi(\boldsymbol{\lambda}^{t+1}) + 
\frac{L}{2} \| \boldsymbol{\lambda} - \mathbf{z}^t \|_2^2 +
\alpha_{t+1} 
\evv{\langle}
\nabla \varphi(\boldsymbol{\lambda}^{t+1}), \,
\boldsymbol{\lambda} - \mathbf{z}^t
\evv{\rangle}.
\end{equation}
После замены последнего выражения в~\eqref{eq_last_in_lem1} на \eqref{eq_last_eq_lem1}
можно воспользоваться расширенным вариантом
неравенства Фенхеля для сопряжённых функций~\cite{Nest_dis}:
$$
\langle \mathbf{g}, \mathbf{s} \rangle + \frac{\xi}{2} \|\mathbf{s}\|^2 \, \ge \, - \frac{1}{2 \xi} \| \mathbf{g} \|_*^2, \, \mathbf{g} \, \in \, \mathbb{E}^*, \, \,  \mathbf{s} \, \in \, \mathbb{E},
$$
где
$\mathbb{E}$~--- конечномерное вещественное векторное пространство, $\mathbb{E}^*$~--- пространство линейных функций на~$\mathbb{E}$ (двойственное пространство),
норма в двойственном пространстве $\|\mathbf{g}\|_* = 
\max\limits_\mathbf{x} \{ \langle \mathbf{g}, \mathbf{x}\rangle  \, | \, \|\mathbf{x} \|_E = 1 \}$.
В нашем случае $\mathbf{g} = \nabla \varphi (\boldsymbol{\lambda}^{t+1})$,
$\mathbf{s} = \boldsymbol{\lambda} - \mathbf{z}^t$, $\xi = \frac{L}{\alpha_{t+1}}$.
Следовательно, 
\begin{equation}
\label{eq_lem1_after_fen}
\psi_{t+1}(\mathbf{z}^{t+1}) \, \ge \, 
A_{t+1} \varphi(\boldsymbol{\lambda}^{t+1}) - \frac{\alpha_{t+1}^2}{2L}
\|\nabla \varphi(\boldsymbol{\lambda}^{t+1})\|^2_2.
\end{equation}
Для завершения доказательства леммы требуется
показать, что $A_{t+1} \varphi(\mathbf{y}^{t+1})$ 
меньше, чем правая часть неравенства
в~\eqref{eq_lem1_after_fen}.

В силу $L$-гладкости функции $\varphi(\boldsymbol{\lambda})$
(см. Утверждение~\ref{2_cor_sopr})
\begin{align*}
    \varphi(\mathbf{y}^{t+1}) & \, \le \,
\varphi(\boldsymbol{\lambda}^{t+1}) + \langle \nabla \varphi(\boldsymbol{\lambda}^{t+1}), \mathbf{y}^{t+1} - \boldsymbol{\lambda}^{t+1}\rangle + \frac{L}{2}
\| \mathbf{y}^{t+1} - \boldsymbol{\lambda}^{t+1} \|_2^2 = \\ &
=\min_{\boldsymbol{\lambda}}
\left \{ \varphi(\boldsymbol{\lambda}^{t+1}) + \langle \nabla \varphi (\boldsymbol{\lambda}^{t+1}) , \boldsymbol{\lambda} - \boldsymbol{\lambda}^{t+1}\rangle  + \frac{L}{2} \| \boldsymbol{\lambda} - \boldsymbol{\lambda}^{t+1} \|_2^2 
			\right
			\}\\ &  =
\varphi(\boldsymbol{\lambda}^{t+1}) - \frac{1}{2 L} \| \nabla \varphi (\boldsymbol{\lambda}^{t+1}) \|_2^2.		
\end{align*}
После умножения обеих частей полученного неравенства на $A_{t+1}$:
$$
A_{t+1} \varphi(\mathbf{y}^{t+1}) \, \le \, A_{t+1} \varphi(\boldsymbol{\lambda}^{t+1}) - \frac{A_{t+1}}{2 L} \| \nabla \varphi (\boldsymbol{\lambda}^{t+1}) \|_2^2.
$$
В силу того, что для коэффициентов БГМ $\alpha_{t+1}^2 \, \le \, A_{t+1}$, получаем
\begin{equation}
\label{eq_aphi_alam}
A_{t+1} \varphi(\mathbf{y}^{t+1}) \, \le \, 
A_{t+1} \varphi(\boldsymbol{\lambda}^{t+1}) - \frac{\alpha_{t+1}^2}{2L}
\|\nabla \varphi(\boldsymbol{\lambda}^{t+1})\|^2_2.
\end{equation}
Следовательно, в силу~\eqref{eq_lem1_after_fen} и \eqref{eq_aphi_alam}
$A_{t+1} \varphi(\mathbf{y}^{t+1}) \, \le \, \psi_{t+1}(\mathbf{z}^{t+1})$,
что и требовалось доказать.~$\blacksquare$

\textbf{Доказательство леммы~\ref{lem_est_1}}
Определим следущее множество: %\pd{Кажется какая-то путаница с $R$ и $\hat{R}$.}
$$
    \Lambda_{2\hat R} = \{\boldsymbol{\lambda} \in \mathbb{R}_{+}^m: \|\boldsymbol{\lambda}\|_2 \leq 2\hat R \}.
$$
%где
\evv{$\hat R$ определяется в силу следующих неравенств:}
$$
||\boldsymbol{\lambda}^0-\boldsymbol{\lambda}^*||_2 + ||\boldsymbol{\lambda}^0||_2 \leq ||\boldsymbol{\lambda}^*||_2 + 2||\boldsymbol{\lambda}^0||_2 \leq 3 R = \hat R.
$$ 
При этом все $\boldsymbol{\lambda}^t$ будут принадлежать $\Lambda_{2\hat R}$, так как 
\begin{align*}
    ||\boldsymbol{\lambda}^t||_2 &\leq ||\boldsymbol{\lambda}^t-\boldsymbol{\lambda}^*||_2 + ||\boldsymbol{\lambda}^* - \boldsymbol{\lambda}^0||_2+||\boldsymbol{\lambda}^0||_2 \\ &\leq  2||\boldsymbol{\lambda}^* - \boldsymbol{\lambda}^0||_2+||\boldsymbol{\lambda}^0||_2 \evv{\, \leq \, } 2||\boldsymbol{\lambda}^*||_2 + 3||\boldsymbol{\lambda}^0||_2 \evv{\, \leq \, } 5 R \leq 2\hat R,
\end{align*}
где для второго неравенства учитывалось, что $||\boldsymbol{\lambda}^t-\boldsymbol{\lambda}^*||_2 \leq ||\boldsymbol{\lambda}^* - \boldsymbol{\lambda}^0||_2$,
\evv{$t = 0, \, 1, \, \ldots$}
\footnote{\evv{Докажем данное неравенство. 
Для любого $\boldsymbol{\lambda} \, \in \, \RR_{+}^m$ в силу
леммы~\ref{lem_fgm_pd}
и сильной выпуклости
функции $\psi_t(\boldsymbol{\lambda})$
с константой $L$ 
верно
\begin{equation}
\label{ap_eq_lam_bound1}
A_t \varphi(\mathbf{y}^t) + \frac{L}{2} \|  
\boldsymbol{\lambda} - \mathbf{z}^t\|_2^2
\, \le \, 
\psi_t(\mathbf{z}^t) +
 \frac{L}{2} \|  
\boldsymbol{\lambda} - \mathbf{z}^t \|_2^2
\, \le \,
\psi_t(\boldsymbol{\lambda}) 
= 
\sum\limits_{j = 0}^t \alpha_j \left [ 
\varphi(\boldsymbol{\lambda}^j) + \langle
			\nabla \varphi (\boldsymbol{\lambda}^j), \boldsymbol{\lambda} - \boldsymbol{\lambda}^j\rangle 
			\right ] 
			+
 \frac{L}{2} \|  
\boldsymbol{\lambda} - \boldsymbol{\lambda}^0 \|_2^2.
\end{equation}
Последнее выражение в~\eqref{ap_eq_lam_bound1} 
в силу выпуклости функции $\varphi(\boldsymbol{\lambda})$
можно
оценить сверху как 
$A_t \varphi (\boldsymbol{\lambda}) +
 \frac{L}{2} \|  
\boldsymbol{\lambda} - \boldsymbol{\lambda}^0 \|_2^2$.
Тогда при $\boldsymbol{\lambda} =
\boldsymbol{\lambda}^*$
$$
\frac{L}{2} \|  
\boldsymbol{\lambda}^* -
\mathbf{z}^t\|_2^2 
\, \le \, 
A_t \left ( 
\varphi(\mathbf{y}^t) - \varphi (\boldsymbol{\lambda}^*) 
\right )
+ \frac{L}{2} \|  
\boldsymbol{\lambda}^* -
\mathbf{z}^t\|_2^2
\, \le \, 
\frac{L}{2} \|  
\boldsymbol{\lambda}^* - \boldsymbol{\lambda}^0 \|_2^2.
$$
Следовательно,
\begin{equation}
\label{ap_eq_lam_bound2}
    \|  
\boldsymbol{\lambda}^* -
\mathbf{z}^t\|_2
\, \le \,
\|  
\boldsymbol{\lambda}^* - \boldsymbol{\lambda}^0 \|_2.
\end{equation}
Поскольку $\mathbf{y}^t$
в Алгоритме~\ref{alg_fgm}
определяется с помощью
шага метода проекции градиента
для выпуклой функции
$\varphi(\boldsymbol{\lambda})$,
последовательность генерируемых
алгоритмом точек
$\mathbf{y}^t$, $t = 0, \, 1, \, \ldots$ также будет
ограничена (доказательство этого
факта см., например, в~\cite[Лемма~9.17, стр.~183]{beck_matlab}
или в~\cite[стр.~265]{bubeck}):
\begin{equation}
\label{ap_eq_lam_bound3}
    \|  
\boldsymbol{\lambda}^* -
\mathbf{y}^t\|_2
\, \le \,
\|  
\boldsymbol{\lambda}^* - \boldsymbol{\lambda}^0 \|_2.
\end{equation}
Далее
$$
\|  
\boldsymbol{\lambda}^{t+1} -
\boldsymbol{\lambda}^{*}\|_2
=
\|  
\tau_t ( \mathbf{z}^t -
\boldsymbol{\lambda}^{*}) +
(1 - \tau_t) 
(\mathbf{y}^t -
\boldsymbol{\lambda}^{*})
\|_2
\, \le \,
\tau_t \| \mathbf{z}^t -
\boldsymbol{\lambda}^{*} \|_2
+
(1 - \tau_t) 
\| \mathbf{y}^t -
\boldsymbol{\lambda}^{*})
\|_2.
$$
Из последнего неравенства
с помощью~\eqref{ap_eq_lam_bound2}, \eqref{ap_eq_lam_bound3}
получаем нужный результат:
$$
\|  
\boldsymbol{\lambda}^{t+1} -
\boldsymbol{\lambda}^{*}\|_2
\, \le, 
\|  
\boldsymbol{\lambda}^{*} -
\boldsymbol{\lambda}^{0}\|_2,
\, t = -1, \, 0, \, 1, \, \ldots
\quad \quad \quad \blacksquare
$$
}}.
%------------------------
В силу леммы~\ref{lem_fgm_pd}
\begin{eqnarray*}
A_N \varphi(\mathbf{y}^N) &  \le & \min_{\boldsymbol{\lambda} \, \in \, 
\RR_+^m} 
\left \{
\frac{L}{2} \|\boldsymbol{\lambda} - \boldsymbol{\lambda}^0\|_2^2 +
\sum\limits_{t = 0}^N \alpha_t \left [ 
\varphi(\boldsymbol{\lambda}^t) + 
			\langle 
			\nabla \varphi (\boldsymbol{\lambda}^t), \boldsymbol{\lambda} - \boldsymbol{\lambda}^t \rangle
			\right ] 
\right \} \, \\
& \le &
\min_{\boldsymbol{\lambda} \, \in \, 
\Lambda_{2\hat R}} 
\left \{
\frac{L}{2} \|\boldsymbol{\lambda} - \boldsymbol{\lambda}^0\|_2^2 +
\sum\limits_{t = 0}^N \alpha_t \left [ 
\varphi(\boldsymbol{\lambda}^t) + 
			\langle 
			\nabla \varphi (\boldsymbol{\lambda}^t), \boldsymbol{\lambda} - \boldsymbol{\lambda}^t \rangle
			\right ] 
\right \} \,\\ &
\overset{\circledOne}{\le} &
 \min_{\boldsymbol{\lambda} \, \in \, 
\Lambda_{2\hat R}}
\left \{
\sum\limits_{t = 0}^N \alpha_t \left [ 
\varphi(\boldsymbol{\lambda}^t) + \langle 
			\nabla \varphi (\boldsymbol{\lambda}^t), \boldsymbol{\lambda} - \boldsymbol{\lambda}^t \rangle
			\right ] 
\right \} +  \frac{ 37L\hat R^2}{9},
\end{eqnarray*}
где $\circledOne$ выполняется, так как
\begin{equation}
\label{eq_fgm_ll0}
\|\boldsymbol{\lambda} - \boldsymbol{\lambda}^0\|^2 \, \le \,
2 \|\boldsymbol{\lambda}\|^2 + 2 \|\boldsymbol{\lambda}^0\|^2 \, \le \, 
8 \hat R^2 + \frac{2}{9} \hat R^2 = \frac{74}{9} \hat R^2. 
\end{equation}
После подстановки определений двойственной целевой
функции $\varphi(\boldsymbol{\lambda}^t)$~\eqref{eq_phi_first} и её градиента~$\nabla \varphi(\boldsymbol{\lambda}^t)$ (см. Утверждение~\ref{2_cor_dem}):
\begin{align*}
\sum\limits_{t = 0}^N & \alpha_t \left [ 
\varphi(\boldsymbol{\lambda}^t) + 
			\langle 
			\nabla \varphi (\boldsymbol{\lambda}^t), \boldsymbol{\lambda} - \boldsymbol{\lambda}^t \rangle
			\right ] \\ & = 
\sum\limits_{t = 0}^N \alpha_t
\left (
\langle \boldsymbol{\lambda}^t, \mathbf{b} \rangle + \sum_{k = 1}^n  \left ( u_k(x^t_k(\boldsymbol{\lambda}^t)) - \langle \boldsymbol{\lambda}^t, \mathbf{C}_k x_k^t(\boldsymbol{\lambda}^t) \rangle\right ) + \langle\mathbf{b} - \sum_{k = 1}^n \mathbf{C}_k x_k^t(\boldsymbol{\lambda}^t) ,
 \boldsymbol{\lambda} - \boldsymbol{\lambda}^t \rangle
\right )  \\ &=   
\sum\limits_{t = 0}^N \alpha_t
\left (
\sum_{k = 1}^n u_k(x_k^t(\boldsymbol{\lambda}^t)) +
 \langle \boldsymbol{\lambda},  \mathbf{b} - \sum_{\evv{k} = 1}^n \mathbf{C}_\evv{k} x_k^t(\boldsymbol{\lambda}^t) \rangle
\right )
 \\ &  \le \,
%\,  \overset{\circledTwo}{\le}
A_N \left (
U(\mathbf{\hat{x}}^{N}) + \langle \boldsymbol{\lambda} , \mathbf{b} -  C\mathbf{\hat{x}}^N \rangle
\right ), 
\end{align*}
где последнее неравенство выполняется в силу вогнутости функций полезности.

Итак, %\pd{Кажется какая-то путаница с $R$ и $\hat{R}$.}
\begin{align*}
A_N \varphi(\mathbf{y}^N) \, & \le \, A_N U(\mathbf{\hat{x}}^{N}) +
\frac{ 37L\hat R^2}{9} +
A_N \min_{\boldsymbol{\lambda} \, \in \, 
\Lambda_{2 \hat R}} 
\left \{ \langle
\boldsymbol{\lambda}, \mathbf{b} -  C\mathbf{\hat{x}}^N \rangle
\right \} \\ &
= A_N U(\boldsymbol{\hat{x}}^{N}) +
\frac{ 37L\hat R^2}{9} -
A_N \max_{\boldsymbol{\lambda} \, \in \, 
\Lambda_{2 \hat R}} 
\left \{\langle
\boldsymbol{\lambda}, C \mathbf{\hat{x}}^N - \mathbf{b} \rangle
\right \} \\
& = A_N U(\boldsymbol{\hat{x}}^{N}) +
\frac{ 37L\hat R^2}{9}- 2 \hat R \pd{A_N} \left \|\left ( C \mathbf{\hat{x}}^N - \mathbf{b}\right )_+ \right \|_2.
\end{align*}
Из этого получаем оценку \eqref{eq_aur37}. ~$\blacksquare$

%%%%%%%%%%%%%%%%%%%%%%%%%%%%%%%%%%%%%%%%%%%%
%
%ЛЕММА 2 СТОХ МЕТОД
%%%%%%%%%%%%%%%%%%%%%%%%%%%%%%%%%%%%%%%%%%%
\subsection{Доказательство леммы~\ref{lem_stoch_main}}

Для доказательства леммы~\ref{lem_stoch_main} сначала приведём доказательства нескольких вспомогательных технических лемм.
\begin{Lem}\label{lem:new_recurrence_lemma_appendix}
     Пусть $A, B$ и $\{r_t\}_{t=0}^N$~--- неотрицательные числа, такие, что для любого $l = 1, \, \ldots, \, N$ выполняется неравенство
    \begin{equation}\label{eq:new_bound_for_r_l_appendix}
         \frac{1}{2} r_l^2 \, \le \, A r_0^2 + B r_0\sqrt{\sum\limits_{t=0}^{l-1} r_t^2}.
     \end{equation}
     Тогда 
     \begin{equation}\label{eq:new_recurrence_lemma_appendix}
         r_l \, \le \, C r_0,
     \end{equation}
     где $C$~--- положительная константа, для которой выполняется $C^2 \, \ge \, \max \left \{1, \, 2A + 2BC \sqrt{N} \right \}$, т.е., в частности, можно выбрать $C = \max \left \{1, \, B\sqrt{N} + \sqrt{B^2N + 2A} \right \}$.
\end{Lem}
\textbf{Доказательство.}
  Докажем \eqref{eq:new_recurrence_lemma_appendix} по индукции. Для $l=0$ неравенство выполнено, так как $C \, \ge \, 1$. Пусть \eqref{eq:new_recurrence_lemma_appendix} выполнено для всех $l < N$. Докажем,
  что оно выполнено и для $l+1$. Действительно,
     \begin{eqnarray*}
        r_{l+1} \,  \overset{\eqref{eq:new_bound_for_r_l_appendix}}{\le} \, 
        \sqrt{2}\sqrt{Ar_0^2 + B r_0\sqrt{\sum\limits_{t=0}^{l}r_t^2}}
    \,    \overset{\eqref{eq:new_recurrence_lemma_appendix}}{\le} \,
        r_0\sqrt{2}\sqrt{A + B C \sqrt{N}}
        = 
        r_0\underbrace{\sqrt{2A + 2 B C \sqrt{N}}}_{\le \, C} \, \le \, Cr_0. \quad \blacksquare
     \end{eqnarray*}

\begin{Lem}
\label{lem_tail_est}
Пусть для последовательностей неотрицательных коэффициентов $\{R_t\}_{t \, \ge \, 0}$ и случайных векторов $\{ \boldsymbol{\eta}^t\}_{t \, \ge \, 0}$,  $\{\mathbf{a}^t\}_{t \, \ge \, 0}$  для всех $l = 1, \, \ldots, \, N$ выполняется неравенство
   \begin{eqnarray}
        \frac{1}{2}R_l^2 \le A + u\sum\limits_{t=0}^{l-1}\langle \boldsymbol{\eta}^t, \, \mathbf{a}^t\rangle,
        \label{eq:radius_recurrence_appendix}
    \end{eqnarray}
    где  $A$~--- неотрицательная константа, $d \, \ge \, 1$~--- положительная константа,
    $\|\mathbf{a}^t\|_2 \, \le \, \widetilde{R}_t d$ и $\widetilde{R}_t = \max \left \{\widetilde{R}_{t-1}, \, R_t \right \}$ для всех $t \, \ge \, 1$, $\widetilde{R}_0 = R_0$, $\widetilde{R}_t$ зависит только от  $\boldsymbol{\eta}^0, \, \ldots, \, \boldsymbol{\eta}^t$. Пусть также вектор $\mathbf{a}^t$~\ev{---} это функция от  $\boldsymbol{\eta}^0, \, \ldots, \, \boldsymbol{\eta}^{t-1}$  $\forall \, t \, \ge \, 1$, $a^0$~\ev{---} постоянный вектор  и для любого $t \, \ge \, 0$ 
    \begin{eqnarray*}
\EE\left[\boldsymbol{\eta}^t\mid \{\boldsymbol{\eta}^k\}_{k=0}^{t-1}\right] = 0,\quad 
\EE\left[\exp\left({\|\boldsymbol{\eta}^t\|_2^2}{\sigma^{-2}}\right)\mid\{\boldsymbol{\eta}^k\}_{k=0}^{t-1}\right] \le \exp(1). \label{eq:eta_k_properties_appendix}
    \end{eqnarray*}
%\ev{$\sigma^2 \leq \frac{\varepsilon}{\ln ( N / \delta )}$.} 
\ev{Т}огда с вероятностью $1 - 2\delta$ выполняются  следующие неравенства:
  \begin{eqnarray*}
        \widetilde{R}_l \le JR_0 \quad \text{ и }\label{eq:tails_estimate_radius_appendix} \quad
        A + u\sum\limits_{t=0}^{l-1}\langle \boldsymbol{\eta}^t, \mathbf{a}^t \rangle \le A + udD\sqrt{\sigma^2 g(N)NJ}\widetilde{R}_0^2
  \end{eqnarray*}
$\forall \, \, l=1, \, \ldots, \, N$ одновременно, где $D$~\ev{---} положительная константа, 
$$
\ev{F} = 2\sigma^2d^2 N (2ud)^{N}\left(2A + ud \widetilde{R}_0^2 + 12 ud \ln\frac{N}{\delta} \sigma^2 N \right),
$$
$\ev{f}=d^2\sigma^2\widetilde{R}_0^2$, $g(N) = \ln\left(\frac{N}{\delta}\right) + \ln\ln\left(\frac{\ev{F}}{\ev{f}}\right)$ и 
$$
J = \max\left\{1, \, \frac{1}{\widetilde{R}_0}udD\sqrt{\sigma^2 g(N)} + \sqrt{\frac{1}{\widetilde{R}_0^2}u^2d^2 C_1^2\sigma^2g(N) + \frac{2A}{R_0^2} }\right\}.$$
\end{Lem}
\textbf{Доказательство.}
Применим ко второму слагаемому из правой части \eqref{eq:radius_recurrence_appendix} неравенство Коши-Буняковского\ev{:}
  \begin{eqnarray}\label{eq:radius_recurrence2}
        \frac{1}{2}R_l^2 \, \le \,  A + ud\sum\limits_{t=0}^{l-1}\|\boldsymbol{\eta}^t\|_2\widetilde{R}_t \, \le \,  A + \frac{ud}{2}\sum\limits_{t=0}^{l-1}\widetilde{R}_t^2 + \frac{ud}{2}\sum\limits_{t=0}^{l-1}\|\boldsymbol{\eta}^t\|_2^2.
    \end{eqnarray}
    
По теореме~2.1 из~\cite{JudNem}
\evv{
\begin{equation}
\label{app_eq_JudNem}
(\forall \, N \, \ge \, 1, \, \forall
\, \gamma \, \ge \, 0): \quad
\mathbb{P} 
\left \{ 
\left \| \sum\limits_{t=0}^{N-1} \boldsymbol{\eta}^t \right \|_2 \, \ge \,
(\sqrt{2} + \sqrt{2} \gamma) \sqrt{ \sum\limits_{t=0}^{N-1} \sigma_t^2} 
%\, | \,
%\{\boldsymbol{\eta}^t\}_{t=0}^{N-1} 
\right \} \, \le \,
\exp \left(-\frac{\gamma^2}{3} \right ).
\end{equation}
Тогда с вероятностью не меньшей, чем
\begin{equation}
\label{app_eq_gamma}
1 - \frac{\delta}{N} = 1 - \exp \left(-\frac{\gamma^2}{3} \right )
\end{equation}
}
выполняется следующее неравенство 
\begin{eqnarray}
\label{app_eq_eta_t}
        \|\boldsymbol{\eta}^t\|_2 \le \sqrt{2}\left(1 + \sqrt{3\ln\frac{N}{\delta}}\right)\sigma \le  2\sqrt{6\ln\frac{N}{\delta}}\sigma.
\end{eqnarray}
\evv{Действительно, выражая из~\eqref{app_eq_gamma} $\gamma$,
получаем, что $\gamma = \sqrt{3\ln\frac{N}{\delta}}$.
Поcле подстановки данного
выражения в~\eqref{app_eq_JudNem}
и выбора единого $\sigma \, \in \, \RR_+$
вместо последовательности $\sigma_t$, $t = 0, \, \ldots, \, N-1$, получаем оценку~\eqref{app_eq_eta_t}.}
%где в последнем неравенстве использовалась оценка $\ln\frac{N}{\delta} \ge 3$.

Объединяя полученные неравенства, получаем\ev{,} что с вероятностью\ev{, большей или равной}~$1 - \delta$ неравенство 
\begin{eqnarray*}
        \frac{1}{2}R_l^2  \le  A + \frac{ud}{2}\sum\limits_{t=0}^{l-1}\widetilde{R}_t^2 + 12 ud \ln\frac{N}{\delta} \sigma^2 l
    \end{eqnarray*}
выполняется для всех $l = 1, \, \ldots, \, N$ одновременно. Заметим, что последнее слагаемое в полученной оценк\ev{е~---}  неубывающая функция от $l$. Определим $\hat l$ как наибольшее целое число\ev{,} для которого выполнено $\hat l \leq l$ и $\widetilde{R}_{\hat{l}} = R_{\hat{l}}$. Тогда получаем, что $R_{\hat{l}} = \widetilde{R}_{\hat{l}} = \widetilde{R}_{\hat{l}+1} = \ldots = \widetilde{R}_{l}$ и\ev{,} следовательно\ev{,} с вероятностью $\ge 1 - \delta$
    \begin{eqnarray*}
        \frac{1}{2}\widetilde{R}_l^2 \le A + \frac{ud}{2}\sum\limits_{t=0}^{\hat{l}-1}\widetilde{R}_t^2 + 12 ud \ln\frac{N}{\delta} \sigma^2 \hat{l}
        \le  A + \frac{ud}{2}\sum\limits_{t=0}^{l-1}\widetilde{R}_t^2 + 12 ud \ln\frac{N}{\delta} \sigma^2 l \quad \forall \, \, l=1, \, \ldots, \, N.
    \end{eqnarray*}
Получаем\ev{,} что с вероятностью $\ge 1 - \delta$ верна следующая оценка 
 \begin{eqnarray*}
        \widetilde{R}_l^2 &\le& 2A + ud\sum\limits_{t=0}^{l-1}\widetilde{R}_k^2 + 24 ud \ln\frac{N}{\delta} \sigma^2 l \\ 
        &\le& 2A\underbrace{(1+ud)}_{\le 2ud} + \underbrace{(ud + u^2d^2)}_{\le 2u^2d^2}\sum\limits_{t=0}^{l-2}\widetilde{R}_t^2 + 24 ud \ln\frac{N}{\delta} \sigma^2\underbrace{( l+ud(l-1))}_{\leq 2udl} \notag\\
        &\le& 2ud\left(2A + ud\sum\limits_{t=0}^{l-2}\widetilde{R}_t^2 + 24 ud \ln\frac{N}{\delta} \sigma^2 l \right),\quad \forall \, \, l = 1, \, \ldots, \, N.\notag
    \end{eqnarray*}
Применяя данную оценку рекурс\ev{и}вно\ev{,} получаем, что с вероятностью $\ge 1 - \delta$ верно
$$
\widetilde{R}_l^2 \le (2ud)^{l}\left(2A + ud \widetilde{R}_0^2 + 24 ud \ln\frac{N}{\delta} \sigma^2 l \right).
$$
Далее рассмотрим последовательность случайных вел\ev{и}чин $\xi^t = \langle \boldsymbol{\eta}^t, \, \mathbf{a}^t \rangle$. Зам\ev{e}тим, что  $\EE\left[\xi^t\mid \xi^0, \, \ldots, \, \xi^{t-1}\right] = \left\langle \EE\left[\boldsymbol{\eta}^t\mid \boldsymbol{\eta}^0, \, \ldots, \, \boldsymbol{\eta}^{k-1}\right], \, \mathbf{a}^t \right\rangle = 0$\ev{,} тогда\ev{,} используя неравенство Коши-Буняковского\ev{,} получаем, что 
 \begin{eqnarray*}
        \EE\left[\exp\left(\frac{(\xi^t)^2}{\sigma^2d^2\widetilde{R}_t^2}\right)\mid \xi^0, \, \ldots, \, \xi^{t-1}\right] &\le& \EE\left[\exp\left(\frac{\|\boldsymbol{\eta}^t\|_2^2 d^2\widetilde{R}_t^2}{\sigma^2 d^2\widetilde{R}_t^2}\right)\mid \boldsymbol{\eta}^0, \, \ldots, \, \boldsymbol{\eta}^{t-1}\right]\\
        &=& \EE\left[\exp\left(\frac{\|\boldsymbol{\eta}^t\|_2^2}{\sigma^2}\right)\mid \boldsymbol{\eta}^0, \, \ldots, \, \boldsymbol{\eta}^{t-1}\right] \, \le \, \exp(1).
    \end{eqnarray*}
Определим $\hat\sigma_t^2 = \sigma^2d^2\widetilde{R}_t^2$, тогда с вероятностью $\ge 1 - \delta$ выполняется 
\begin{eqnarray*}
 \sum\limits_{t=0}^{l-1} \hat\sigma_t^2 & \leq  &\sigma^2d^2 l (2ud)^{l}\left(2A + ud \widetilde{R}_0^2 + 24 ud \ln\frac{N}{\delta} \sigma^2 l \right) \\ & \leq& \sigma^2d^2 N (2ud)^{N}\left(2A + ud \widetilde{R}_0^2 + 24 ud \ln\frac{N}{\delta} \sigma^2 N \right) := \dfrac{\ev{F}}{2},
 \end{eqnarray*}
для всех  $l = 1, \, \ldots, \, N$ одновременно, где $\ev{F} = 2\sigma^2d^2 N (2ud)^{N}\left(2A + ud \widetilde{R}_0^2 + 24 ud \ln\frac{N}{\delta} \sigma^2 N \right)$. 

Используя следствие~8 из \cite{jin2019short} для $b=\hat\sigma_0^2$\ev{,} получаем для любого $l=1, \, \ldots, \, N$ с вероятностью $\ge 1-\frac{\delta}{N}$ следующую оценку
    \begin{equation}
    \label{ap_eq_libo}
        \text{либо } \sum\limits_{t=0}^{l-1}\hat\sigma_t^2 \ge \ev{F}, \text{ либо } \left|\sum\limits_{t=0}^{l-1}\xi^t\right| \le C_1\sqrt{\sum\limits_{t=0}^{l-1}\hat\sigma_t^2\left(\ln\left(\frac{N}{\delta}\right) + \ln\ln\left(\frac{\ev{F}}{\ev{f}}\right)\right)},
    \end{equation}
где $C_1 >0$~\ev{---} константа, которая не зависит от $\ev{F}$ и $\ev{f}$. 

Далее\ev{,} объединяя полученные оценки\ev{,} получаем, что
\evv{оценка~\eqref{ap_eq_libo}}
с вероятностью $\ge 1-\delta$ 
\evv{верна } 
%\begin{equation*}
 %       \text{либо } %\sum\limits_{t=0}^{l-1}\hat\sigma_t^2 \ge \ev{F}, %\text{ либо } %\left|\sum\limits_{t=0}^{l-1}\xi^t\right| \le %C_1\sqrt{\sum\limits_{t=0}^{l-1}\hat\sigma_t^2\left(\l%n\left(\frac{N}{\delta}\right) + %\ln\ln\left(\frac{\ev{F}}{\ev{f}}\right)\right)}
 %   \end{equation*}
 для всех  $l=1, \, \ldots, \, N$ одновременно. 
 
 Учитывая выбор $\ev{F}$\ev{,} получаем, что с вероятностью $\ge 1-2\delta$
\begin{equation*}
\left|\sum\limits_{t=0}^{l-1}\xi^t\right| \le C_1\sqrt{\sum\limits_{t=0}^{l-1}\hat\sigma_t^2\left(\ln\left(\frac{N}{\delta}\right) + \ln\ln\left(\frac{\ev{F}}{\ev{f}}\right)\right)}
    \end{equation*}
    для всех  $l=1, \, \ldots, \, N$ одновременно. 
    
    Для удобства дальнейших рассуждений обозначим $g(N) := \ln\left(\frac{N}{\delta}\right) + \ln\ln\left(\frac{\ev{F}}{\ev{f}}\right) \approx \ln\left(\frac{N}{\delta}\right) $, пр\ev{е}небрегая константой. Использу\ev{я} $\hat\sigma_t^2 = \sigma^2d^2\widetilde{R}_t^2$\ev{,}  получаем, что с вероятностью $\ge 1-2\delta$ справедлива следующая оценка\ev{:} 
 \begin{eqnarray}
        \frac{1}{2}\widetilde{R}_l^2 &\le& A + u\sum\limits_{t=0}^{l-1}\underbrace{\langle \boldsymbol{\eta}^t, \, \mathbf{a}^t\rangle }_{\xi^t}
    \,    \le \, A + udD\sqrt{\sigma^2 g(N)}\sqrt{\sum\limits_{t=0}^{l-1}\widetilde{R}_t^2}\notag\\
\end{eqnarray}
для всех  $l=1, \, \ldots, \, N$ одновременно. Выбирая в качестве $A=\frac{A}{\widetilde{R}_0^2}$\ev{,}  $B =\frac{1}{\widetilde{R}_0}udC_1\sqrt{\sigma^2 g(N)}$, $r_t = \widetilde{R}_t $\ev{,} из леммы~\ref{lem:new_recurrence_lemma_appendix} получаем\ev{,} что с вероятностью  $1-2\delta$ выполняется 
    \begin{eqnarray*}
        \widetilde{R}_l \le JR_0
    \end{eqnarray*}
    для всех $l=1, \, \ldots, \, N$ одновременно, где  
    $$
    J = \max\left\{1, \, \frac{1}{\widetilde{R}_0}udC_1\sqrt{\sigma^2 g(N)} + \sqrt{\frac{1}{\widetilde{R}_0^2}u^2d^2C_1^2\sigma^2g(N) + \frac{2A}{R_0^2} }\right\}.
    $$ 
    Отсюда получаем, что с вероятностью $1-2\delta$ оценка
 \begin{eqnarray*}
         A + u\sum\limits_{t=0}^{l-1}\langle \boldsymbol{\eta}^t, \mathbf{a}^t\rangle
        \le A + udC_1\sqrt{\sigma^2 g(N)lJ}\widetilde{R}_0^2 \le A + udC_1\sqrt{\sigma^2 g(N)NJ}\widetilde{R}_0^2\notag\\
\end{eqnarray*}
\ev{верна} для всех  $l=1, \, \ldots, \, N$ одновременно. 
~$\blacksquare$

\textbf{Доказательство леммы~\ref{lem_stoch_main}}

Для $\boldsymbol{\lambda} \, \in \, \RR_+^m$ 
$$
\| \boldsymbol{\lambda}^{t+1} - \boldsymbol{\lambda} \|_2^2 =
\|
[\boldsymbol{\lambda}^t - \beta \nabla \varphi(\boldsymbol{\lambda}^t, \, \xi^t)]_+ - \boldsymbol{\lambda} \|_2^2 \, \le \,
\| \boldsymbol{\lambda}^t - \boldsymbol{\lambda} \|_2^2 - 
2 \beta \langle \nabla \varphi(\boldsymbol{\lambda}^t, \, \xi^t),
\boldsymbol{\lambda}^t - \boldsymbol{\lambda}\rangle + \beta^2 
\| \nabla \varphi(\boldsymbol{\lambda}^t, \, \xi^t) \|_2^2,
$$
т.е. 
\begin{equation}
\label{eq_stoch_t1}
0 \, \le \, \frac{1}{2 \beta}
\left (
\| \boldsymbol{\lambda}^t - \boldsymbol{\lambda} \|_2^2 -
\| \boldsymbol{\lambda}^{t+1} - \boldsymbol{\lambda} \|_2^2 
\right ) +
\langle \nabla \varphi(\boldsymbol{\lambda}^t, \, \xi^t),
\boldsymbol{\lambda} - \boldsymbol{\lambda}^t \rangle +
\frac{\beta}{2} 
\| \nabla \varphi(\boldsymbol{\lambda}^t, \, \xi^t) \|_2^2.    
\end{equation}
После прибавления к обеим сторонам неравенства~\eqref{eq_stoch_t1} $\varphi(\boldsymbol{\lambda}^t)$, умножения на $N$
и суммирования от $0$ до $N-1$:
\begin{align}
\label{eq:1}
\dfrac{1}{N}\sum_{t = 0}^{N-1} \varphi(\boldsymbol{\lambda}^t) & \, \le \,
\dfrac{1}{N} \sum_{t = 0}^{N-1} 
\Bigg \{
\varphi(\boldsymbol{\lambda}^t) +
\langle \nabla \varphi(\boldsymbol{\lambda}^t, \, \xi^t), \,
\boldsymbol{\lambda} - \boldsymbol{\lambda}^t\rangle +
\frac{\beta}{2} 
\| \nabla \varphi(\boldsymbol{\lambda}^t, \, \xi^t) \|_2^2 \notag \\ &
+ \frac{1}{2 \beta}
\Big (
\| \boldsymbol{\lambda}^t - \boldsymbol{\lambda} \|_2^2 -
\| \boldsymbol{\lambda}^{t+1} - \boldsymbol{\lambda} \|^2_2
\Big )
\Bigg \}.
\end{align}
В силу выпуклости $\varphi(\boldsymbol{\lambda})$ 
для $\boldsymbol{\hat{\lambda}}^N = \dfrac{1}{N}\sum\limits_{t=0}^{N-1}
\boldsymbol{\lambda}^t$ получаем, что 
\begin{align}
\label{eq:1}
N  \varphi(\ev{\hat{\boldsymbol{\lambda}}}^N) & \, \le \,
 \sum_{t = 0}^{N-1} 
\left \{
\varphi(\boldsymbol{\lambda}^t) +
\langle \nabla \varphi(\boldsymbol{\lambda}^t, \, \xi^t),
\boldsymbol{\lambda} - \boldsymbol{\lambda}^t\rangle \right \} +
\frac{\beta}{2} 
\| \nabla \varphi(\boldsymbol{\lambda}^t, \, \xi^t) \|_2^2 \notag 
+ \frac{1}{2 \beta}
\Big (
\| \boldsymbol{\lambda}^0 - \boldsymbol{\lambda} \|_2^2 -
\| \boldsymbol{\lambda}^{N} - \boldsymbol{\lambda} \|^2_2
\Big ).
\end{align}
Выбираем $ \boldsymbol{\lambda} =  \boldsymbol{\lambda}^*$ и прибавляем и вычитаем справа $ \sum_{t = 0}^{N-1} \langle \nabla \varphi(\boldsymbol{\lambda}^t), \,
\boldsymbol{\lambda}^* - \boldsymbol{\lambda}^t\rangle$. \ev{П}олучаем 
\begin{eqnarray}
  N  \varphi(\ev{\hat{\boldsymbol{\lambda}}}^N) &  \le &
 \sum\limits_{t = 0}^{N-1} 
\left \{
\varphi(\boldsymbol{\lambda}^t) +
\langle \nabla \varphi(\boldsymbol{\lambda}^t),
\boldsymbol{\lambda}^* - \boldsymbol{\lambda}^t\rangle \right \} +
\frac{\beta}{2} 
\| \nabla \varphi(\boldsymbol{\lambda}^t, \, \xi^t) \|_2^2 \notag \\ & + &  \sum\limits_{t = 0}^{N-1} \langle \nabla \varphi( \boldsymbol{\lambda}^t, \, \xi^t) - \nabla \varphi(\boldsymbol{\lambda}^t),
\boldsymbol{\lambda}^* - \boldsymbol{\lambda}^t\rangle
+ \frac{1}{2 \beta}
\Big (
\| \boldsymbol{\lambda}^0 - \boldsymbol{\lambda}^* \|_2^2 -
\| \boldsymbol{\lambda}^{N} - \boldsymbol{\lambda}^* \|^2_2
\Big )\ev{.}      \label{eq:3}
\end{eqnarray}
Из выпуклости $\varphi(\boldsymbol{\lambda})$ \ev{имеем}%получаем 
\begin{eqnarray*}
 \sum\limits_{t = 0}^{N-1} 
\left \{
\varphi(\boldsymbol{\lambda}^t) +
\langle \nabla \varphi(\boldsymbol{\lambda}^t), \,
\boldsymbol{\lambda}^* - \boldsymbol{\lambda}^t\rangle \right \}\, \le \, \sum\limits_{t = 0}^{N-1} 
\left \{
\varphi(\boldsymbol{\lambda}^t) + \varphi(\boldsymbol{\lambda}^*) - \varphi(\boldsymbol{\lambda}^t) \right \} \leq \sum\limits_{t = 0}^{N-1}  \varphi(\ev{\boldsymbol{\lambda}^*}) \leq N\varphi(\boldsymbol{\lambda}^*).
\end{eqnarray*}
Подставляя полученную оценку в \eqref{eq:3}, получаем 
\begin{eqnarray}
 \frac{1}{2 \beta} \| \boldsymbol{\lambda}^{N} - \boldsymbol{\lambda}^* \|^2_2 \leq 
  \frac{1}{2 \beta} \| \boldsymbol{\lambda}^{0} - \boldsymbol{\lambda}^* \|^2_2 +
 \sum\limits_{t = 0}^{N-1} 
\langle \nabla \varphi( \boldsymbol{\lambda}^t, \, \xi^t) - \nabla \varphi(\boldsymbol{\lambda}^t), \,
\boldsymbol{\lambda}^* - \boldsymbol{\lambda}^t\rangle  +
\frac{\beta}{2} 
\| \nabla \varphi(\boldsymbol{\lambda}^t, \, \xi^t) \|_2^2.   \label{eq:2}
\end{eqnarray}
Определим $R_{t}=\| \boldsymbol{\lambda}^{t} - \boldsymbol{\lambda}^* \|_2$ и $\widetilde{R}_t = \max\{\widetilde{R}_{t-1}, \, R_t\}$, причём $R_0=\widetilde{R}_0$ и\ev{,} так как\ev{,} $ \boldsymbol{\lambda}^{0}=\mathbf{0}$  и $\| \boldsymbol{\lambda}^{*}\|_2 \leq R$, то $R_0=R$. При этом по построению получаем, что $\boldsymbol{\lambda}^{t} \, \in \, B_{\widetilde{R}_t}(\boldsymbol{\lambda}^{*})$. Так же определим $\|\mathbf{a}^t \|_2= \| \boldsymbol{\lambda}^{t} - \boldsymbol{\lambda}^* \|_2 \leq \widetilde{R}_t$. Тогда \eqref{eq:2} можно переписать в следующем виде\ev{:}
\begin{eqnarray*}
 \frac{1}{2 \beta}\widetilde{R}_N^2 \leq 
  \frac{1}{2 \beta} \widetilde{R}_0^2 +
 \sum\limits_{t = 0}^{N-1} 
\langle \nabla \varphi( \boldsymbol{\lambda}^t, \, \xi^t)- \nabla \varphi(\boldsymbol{\lambda}^t), \,
\mathbf{a}^t \rangle  +
\frac{\beta}{2} 
\| \nabla \varphi(\boldsymbol{\lambda}^t, \, \xi^t) \|_2^2.   
\end{eqnarray*}
Обозначим $\boldsymbol{\eta}^t = \nabla \varphi(\boldsymbol{\lambda}^t, \, \xi^t) -
\nabla \varphi(\boldsymbol{\lambda}^t)$.
По теореме~2.1 из~\cite{JudNem}
\begin{eqnarray}
\label{estimation_1}
\mathbb{P} 
\left \{ \left
\| \sum\limits_{t=0}^{N-1} \boldsymbol{\eta}^t \right \|_2 \, \ge \,
(\sqrt{2} + \sqrt{2} \gamma) \sqrt{ \sum\limits_{t=0}^{N-1} \sigma_t^2} \, | \,
\{\xi^t\}_{t=0}^{N-1} 
\right \} \, \le \,
\exp \left(-\frac{\gamma^2}{3} \right ).
\end{eqnarray}
Используя лемму 2 из \cite{jin2019short}, получаем\ev{, что}  $\EE\left[\exp\left({\frac{\|\boldsymbol{\eta}^t\|_2^2}{\sigma^2}}\right)|\{\xi^k\}_{k=0}^{t-1}\right] \le \exp(1)$, при этом %получаем, что 
 $\ev{\mathbf{\eta}}^t$ зависит только от $\xi^{t-1}, \, \ldots, \, \xi^0$. Используя новые обозначения и \eqref{eq_stoch_gradM}, \ev{имеем}%получаем 
\begin{eqnarray*}
\widetilde{R}_N^2 \leq 
 \widetilde{R}_0^2 + 2 \beta
 \sum\limits_{t = 0}^{N-1} 
\langle\boldsymbol{\eta}^t, \,
\mathbf{a}^t \rangle  +
\beta^2 M^2.   
\end{eqnarray*}
Тогда из леммы \ref{lem_tail_est} с константами $A= \widetilde{R}_0^2 + \beta^2 M^2$, $d=1$ и $u =  \beta$, получаем, что с вероя\ev{т}ностью $1-2\delta$,
 \ev{ где~$\frac{\delta}{N} = \exp \left(-\frac{\gamma^2}{3} \right )$,} верна следующая оценка\ev{:} 
 \begin{eqnarray}
  \label{est_part_2}
        \widetilde{R}_l \le JR_0 \quad \text{ и }\label{eq:tails_estimate_radius_appendix} \quad
         \sum\limits_{t=0}^{l-1}\langle \boldsymbol{\eta}^t, \, \mathbf{a}^t \rangle \, \le     \, D\sqrt{\sigma^2 g(N)NJ}\widetilde{R}_0^2
  \end{eqnarray}
$\forall \, l=1, \, \ldots, \, N$ одновременно, где $D$~\ev{---} положительная константа,
$$
\ev{F} = 2\sigma^2 N (2 \beta)^{N}\left(2A +  \beta \widetilde{R}_0^2 + 24 \ln\frac{N}{\delta} \beta \sigma^2 N \right),
$$
$\ev{f}=\sigma^2\widetilde{R}_0^2$, $g(N) = \ln\left(\frac{N}{\delta}\right) + \ln\ln\left(\frac{\ev{F}}{\ev{f}}\right)$ и 
$$
J = \max\left\{1, \, \frac{1}{\widetilde{R}_0} \beta C_1\sqrt{\sigma^2 g(N)} + \sqrt{\frac{1}{\widetilde{R}_0^2} \beta^2 C_1^2\sigma^2g(N) + \frac{2A}{R_0^2} }\right\}.
$$
 
Чтобы оценить зазор двойственности\ev{,} используем \eqref{eq:1}, также отметим, что данная оценка верна для любого $\boldsymbol{\lambda} \, \in \, \RR_+^m$. Поэтому\ev{,} беря минимум по \ev{всем $\boldsymbol{\lambda}$ из множества}  $\Lambda_{2R} =  \{\boldsymbol{\lambda} \, \in \, \mathbb{R}_{+}^m: \|\boldsymbol{\lambda}\|_2 \leq 2 R \}
$, получаем 
\begin{align*}
N \varphi(\boldsymbol{\hat{\lambda}}^N) \,  \le \,
\min_{\boldsymbol{\lambda} \, \in \, \Lambda_{2 R}}
\left \{
\sum_{t = 0}^{N-1} 
\left (
\varphi(\boldsymbol{\lambda}^t) +
\langle \nabla \varphi(\boldsymbol{\lambda}^t, \, \xi^t),
\boldsymbol{\lambda} - \boldsymbol{\lambda}^t \rangle
\right ) +
 \frac{1}{2 \beta}
 \| \boldsymbol{\lambda}^0 - \boldsymbol{\lambda} \|_2^2
\right \}
+ \frac{N\beta M^2}{2},
\end{align*}
где для оценки последнего слагаемого использовалось   \ev{предположение}~\eqref{eq_stoch_gradM}.
Также учитывалось, что $\| \boldsymbol{\lambda}^{N} - \boldsymbol{\lambda} \|^2_2 \geq 0$.
В силу~\eqref{eq_fgm_ll0} получаем следующую оценку\ev{:}
$$
 \varphi(\boldsymbol{\hat{\lambda}}^N)  \, \le \,
 \frac{1}{N}
\min_{\boldsymbol{\lambda} \, \in \, \Lambda_{2R}}
\left \{
\sum_{t = 0}^{N-1} 
\left (
\varphi(\boldsymbol{\lambda}^t) +
\langle \nabla \varphi(\boldsymbol{\lambda}^t, \, \xi^t),
\boldsymbol{\lambda} - \boldsymbol{\lambda}^t \rangle
\right ) 
\right \}
+ 
\frac{2R^2}{ \beta N} +
\frac{\beta M^2}{2}.
$$
Прибавим и вычт\ev{е}м из выражения под минимумом $\sum\limits_{t = 0}^{N-1} \langle \nabla \varphi(\boldsymbol{\lambda}^t), \,
\boldsymbol{\lambda} - \boldsymbol{\lambda}^t \rangle$.
\ev{Тогда} 
\begin{align*}
\min_{\boldsymbol{\lambda} \, \in \, \Lambda_{2 R}} &
\left \{
\sum_{t = 0}^{N-1} 
\left (
\varphi(\boldsymbol{\lambda}^t) +
\langle \nabla \varphi(\boldsymbol{\lambda}^t), \,
\boldsymbol{\lambda} - \boldsymbol{\lambda}^t \rangle
\right ) 
\right \} 
\le \, 
 \min_{\boldsymbol{\lambda} \, \in \, \Lambda_{2 R}} 
\left \{
\sum_{t = 0}^{N-1} 
\left (
\varphi(\boldsymbol{\lambda}^t) +
\langle \nabla \varphi(\boldsymbol{\lambda}^t, \, \xi^t), \,
\boldsymbol{\lambda} - \boldsymbol{\lambda}^t \rangle
\right ) 
\right \} \\&  
+ 
\max_{\boldsymbol{\lambda} \, \in \, \Lambda_{2 R}}
\left \{
\sum_{t = 0}^{N-1} \langle \nabla \varphi(\boldsymbol{\lambda}^t, \, \xi^t)  -
\nabla \varphi(\boldsymbol{\lambda}^t), \,  \boldsymbol{\lambda}\rangle 
\right \}  + \sum_{t = 0}^{N-1} \langle \nabla \varphi(\boldsymbol{\lambda}^t, \, \xi^t) -
\nabla \varphi(\boldsymbol{\lambda}^t), \, - \boldsymbol{\lambda}^t \rangle.
\end{align*}
Заметим, что $ - \boldsymbol{\lambda}^* \, \in \, \Lambda_{2 R}$. Тогда 
\begin{eqnarray*}
\sum_{t = 0}^{N-1} \langle \nabla \varphi(\boldsymbol{\lambda}^t, \, \xi^t) -
\nabla \varphi(\boldsymbol{\lambda}^t), \, - \boldsymbol{\lambda}^t \rangle & = &\sum_{t = 0}^{N-1}  \langle \nabla \varphi(\boldsymbol{\lambda}^t, \, \xi^t) -
\nabla \varphi(\boldsymbol{\lambda}^t), \, \boldsymbol{\lambda}^* - \boldsymbol{\lambda}^t  \rangle \\ 
& + & \sum_{t = 0}^{N-1}  \langle \nabla \varphi(\boldsymbol{\lambda}^t, \, \xi^t) -
\nabla \varphi(\boldsymbol{\lambda}^t), \, - \boldsymbol{\lambda}^* \rangle  \\ 
& \leq &
\max_{\boldsymbol{\lambda} \, \in \, \Lambda_{2 R}}
\sum_{t = 0}^{N-1}
 \langle \nabla \varphi(\boldsymbol{\lambda}^t, \, \xi^t)  -
\nabla \varphi(\boldsymbol{\lambda}^t), \,   \boldsymbol{\lambda}\rangle 
\\
&  + & \sum_{t = 0}^{N-1} \langle \nabla \varphi(\boldsymbol{\lambda}^t, \, \xi^t) - \nabla \varphi(\boldsymbol{\lambda}^t), \, \boldsymbol{\lambda}^* - \boldsymbol{\lambda}^t  \rangle.
\end{eqnarray*}
Отсюда получаем следующую оценку\ev{:} 
\begin{subequations}\label{ap_al_philamn}
\begin{align*}
\begin{split}
 \varphi(\boldsymbol{\hat{\lambda}}^N) &  \, \le \,
 \frac{1}{N}
\min_{\boldsymbol{\lambda} \, \in \, \Lambda_{2R}}
\left \{
\sum_{t = 0}^{N-1} 
\left (
\varphi(\boldsymbol{\lambda}^t) +
\langle \nabla \varphi(\boldsymbol{\lambda}^t, \, \xi^t), \,
\boldsymbol{\lambda} - \boldsymbol{\lambda}^t \rangle
\right ) 
\right \}
+ 
\frac{2 R^2}{ \beta N} +
\frac{\beta M^2}{2}  
\end{split}
\\
\begin{split}
& \leq 
\frac{1}{N}
\min_{\boldsymbol{\lambda} \, \in \, \Lambda_{2 R}}
\left \{
\sum_{t = 0}^{N-1} 
\left (
\varphi(\boldsymbol{\lambda}^t) +
\langle \nabla \varphi(\boldsymbol{\lambda}^t), \,
\boldsymbol{\lambda} - \boldsymbol{\lambda}^t \rangle
\right ) 
\right \}
+ \frac{1}{N} \sum_{t = 0}^{N-1} \langle \nabla \varphi(\boldsymbol{\lambda}^t, \, \xi^t)-  \nabla \varphi(\boldsymbol{\lambda}^t), \, \boldsymbol{\lambda}^* - \boldsymbol{\lambda}^t \rangle \end{split}
\\
\begin{split}
& + 
\frac{2}{N} \max_{\boldsymbol{\lambda} \, \in \, \Lambda_{2 R}}
\left \{
\sum_{t = 0}^{N-1} \langle \nabla \varphi(\boldsymbol{\lambda}^t, \, \xi^t)  -
\nabla \varphi(\boldsymbol{\lambda}^t), \, \boldsymbol{\lambda}\rangle 
\right \}  + 
\frac{2 R^2}{ \beta N} +
\frac{\beta M^2}{2}. 
\end{split}
\tag{\ref{ap_al_philamn}}
\end{align*}
\end{subequations}
Из определения нормы получаем\ev{, что} 
$$
\max_{\boldsymbol{\lambda} \, \in \, \Lambda_{2 R}}
\left \{
\sum_{t = 0}^{N-1} \left \langle \nabla \varphi(\boldsymbol{\lambda}^t, \, \xi^t)  -
\nabla \varphi(\boldsymbol{\lambda}^t), \, \boldsymbol{\lambda} \right \rangle 
\right \} \leq 2 R \left \|
\sum_{t = 0}^{N-1} \left ( 
\nabla \varphi(\boldsymbol{\lambda}^t, \, \xi^t) -
\nabla \varphi(\boldsymbol{\lambda}^\ev{l}) 
\right ) 
\right \|_2.
$$
Используя \eqref{estimation_1}, получаем\ev{,} что с вероятностью $1-\delta$ выполняется 
\begin{equation}
\label{est_part_1}
   \left \|
\sum_{t = 0}^{N-1} 
\left ( 
\nabla \varphi(\boldsymbol{\lambda}^t, \, \xi^t) -
\nabla \varphi(\boldsymbol{\lambda}^\ev{l}) 
\right ) 
\right \|_2 \leq \sigma \sqrt{2 N} 
 \left (1 + \sqrt{3 \ln \frac{1}{\delta}}
 \right ).  
\end{equation}
\evv{Подставим в выражение $\sum\limits_{t = 0}^{N-1} \left (
\varphi(\boldsymbol{\lambda}^t) +
\langle \nabla \varphi(\boldsymbol{\lambda}^t), \,
\boldsymbol{\lambda} - \boldsymbol{\lambda}^t \rangle
\right )$ из
\eqref{ap_al_philamn}
значения $\varphi(\boldsymbol{\lambda}^t)$
 и $\nabla \varphi(\boldsymbol{\lambda}^t)$,
 получим
$$
\sum\limits_{t = 0}^{N-1} \left (
\langle \boldsymbol{\lambda^t}, \mathbf{b} \rangle + \sum_{k = 1}^n (u_k(x_k(\boldsymbol{\lambda^t})) - \langle \boldsymbol{\lambda}^t, \, \mathbf{C}_k x_k(\boldsymbol{\lambda^t}) \rangle ) +
\langle\mathbf{b} - C\mathbf{x}^t (\boldsymbol{\lambda^t}), \,
\boldsymbol{\lambda} - \boldsymbol{\lambda}^t \rangle
\right ) =
$$
$$
= \sum\limits_{t = 0}^{N-1} \left (
\sum_{k = 1}^n (u_k(x_k(\boldsymbol{\lambda^t})) +
\langle\mathbf{b} - C\mathbf{x}^t (\boldsymbol{\lambda^t}), \,
\boldsymbol{\lambda} \rangle
\right ).
$$
Тогда в силу вогнутости функций $u_k(x_k)$
$$
\frac{1}{N}
\min_{\boldsymbol{\lambda} \, \in \, \Lambda_{2 R}}
\left \{
\sum_{t = 0}^{N-1} 
\left (
\varphi(\boldsymbol{\lambda}^t) +
\langle \nabla \varphi(\boldsymbol{\lambda}^t), \,
\boldsymbol{\lambda} - \boldsymbol{\lambda}^t \rangle
\right ) 
\right \}
\leq U(\mathbf{\hat{x}}^N) 
- \frac{1}{N}
\max_{\boldsymbol{\lambda} \, \in \, \Lambda_{2 R}} 
\left \{
\sum_{t = 0}^{N-1} 
\langle  C \mathbf{x}^t(\boldsymbol{\lambda}^t) - \mathbf{b}, \,
\boldsymbol{\lambda} \rangle 
\right \}.
$$
%После подстановки значений $\varphi(\boldsymbol{\lambda}^t)$
% и $\nabla \varphi(\boldsymbol{\lambda}^t)$, учитывая вогнутость функций $u_k(x_k)$\ev{,} 
Учитывая последнее неравенство, из \eqref{ap_al_philamn}
получаем:} 
 \begin{align*}
 \varphi(\boldsymbol{\hat{\lambda}}^N) \, & \le \,
U(\evv{\mathbf{\hat{x}}^N})%   \mathbf{x}(\boldsymbol{\lambda}^N)) 
- \frac{1}{N}
\max_{\boldsymbol{\lambda} \, \in \, \Lambda_{2 R}} 
\left \{
\sum_{t = 0}^{N-1} 
\langle  C \mathbf{x}^t(\boldsymbol{\lambda}^t) - \mathbf{b}, \,
\boldsymbol{\lambda} \rangle 
\right \} + \frac{2R^2}{ \beta N} +
\frac{\beta M^2}{2}
 \\ & 
+ \frac{2 R}{N} 
\left \|
\sum_{t = 0}^{N-1} 
\left ( \nabla \varphi(\boldsymbol{\lambda}^t, \, \xi^t) -
\nabla \varphi(\boldsymbol{\lambda}^t) 
\right ) 
\right \|_2 + \frac{1}{N} \sum_{t = 0}^{N-1} \langle \nabla \varphi(\boldsymbol{\lambda}^t, \, \xi^t)-  \nabla \varphi(\boldsymbol{\lambda}^t), \, \boldsymbol{\lambda}^* - \boldsymbol{\lambda}^t \rangle . 
\end{align*}
Отсюда, учитывая оценк\ev{y} \eqref{est_part_1} и результат~\eqref{estimation_1}, получаем\ev{,} что с вероятностью $1-3\delta$

 \begin{eqnarray}
 \label{part_1}
 \varphi(\boldsymbol{\hat{\lambda}}^N) 
 - U(\mathbf{\hat{x}}^N)  + 
2 R
\left \|
\left [C \hat{\mathbf{x}}^N - \mathbf{b}
\right ]_+ 
\right \|_2  \, & \le & \,  \frac{2 R \sigma \sqrt{2} 
 \left (1 + \sqrt{3 \ln \frac{1}{\delta}}
 \right )}{\sqrt{N}}
+ \frac{2 R^2}{\beta N} +
\frac{\beta M^2}{2}  \notag \\ & + &    C_1\dfrac{\sigma\sqrt{ g(N)J} R ^ 2}{\sqrt{N}}. 
 \end{eqnarray}

По теореме~2.1 из~\cite{JudNem} для всех $\gamma > 0$
\begin{eqnarray*}
\mathbb{P} 
\left \{ 
\left \| \sum\limits_{t=0}^{N-1} \left( \mathbf{x}(\boldsymbol{\lambda}^t, \, \xi^t)-\mathbf{x}(\boldsymbol{\lambda}^t)\right) \right \|_2 \, \ge \,
(\sqrt{2} + \sqrt{2} \gamma) \sqrt{ \sum\limits_{t=0}^{N-1} \sigma_x^2} \, | \,
\{\xi^t\}_{t=0}^{N-1} 
\right \} \, \le \,
\exp \left(-\frac{\gamma^2}{3} \right ).
\end{eqnarray*}
Выбирая $\gamma=\sqrt{3\ln \frac{1}{\delta}}$, получаем\ev{,} что с вероятностью $1 - \delta$
\begin{eqnarray*}
\|\Tilde{\mathbf{x}}^N - \hat{\mathbf{x}}^N \|_2  =  \dfrac{1}{N} \left \| \sum\limits_{t=0}^{N-1} \left( \mathbf{x}(\boldsymbol{\lambda}^t, \xi^t)-\mathbf{x}(\boldsymbol{\lambda}^t)\right) \right \|_2 
 \leq  \sigma_x \sqrt{\frac{2 }{N}} 
 \left (1 + \sqrt{3 \ln \frac{1}{\delta}}
 \right ).
\end{eqnarray*}
Тогда с вероятностью $1 - \delta$ выполняется следующее неравенство\ev{:} 
\begin{eqnarray*}
\|C\Tilde{\mathbf{x}}^N - C\hat{\mathbf{x}}^N \|_2  \leq \|C\|_2\cdot \|\Tilde{\mathbf{x}}^N - \hat{\mathbf{x}}^N \|_2 
 \leq  \sigma_x \sqrt{\frac{2 \lambda_{max}\left( C^{T}C \right)}{N}}
 \left (1 + \sqrt{3 \ln \frac{1}{\delta}}
 \right ).
\end{eqnarray*}
Заметим, что 
\begin{eqnarray}
\label{part_2}
2 R
\left \|
\left [C \Tilde{\mathbf{x}}^N - \mathbf{b}
\right ]_+ 
\right \|_2 & =& \max_{\boldsymbol{\lambda} \, \in \, \Lambda_{2 R}} 
\left \{
\langle  C \Tilde{\mathbf{x}}^N - \mathbf{b}, \,
\boldsymbol{\lambda} \rangle 
 + \langle  C \hat{\mathbf{x}}^N -  C \hat{\mathbf{x}}^N - \mathbf{b} + \mathbf{b}, \,
\boldsymbol{\lambda} \rangle 
\right \} \notag\\
&\leq & 
\max_{\boldsymbol{\lambda} \, \in \, \Lambda_{2 R}} 
\left \{
\langle  C \hat{\mathbf{x}}^N - \mathbf{b}, \,
\boldsymbol{\lambda} \rangle 
\right \} + \max_{\boldsymbol{\lambda} \, \in \, \Lambda_{2 R}} 
\left \{
\langle  C \Tilde{\mathbf{x}}^N -  C \hat{\mathbf{x}}^N, \,
\boldsymbol{\lambda} \rangle 
\right \} \notag
\\
& \leq & 2 R
\left \|
\left [C \hat{\mathbf{x}}^N - \mathbf{b}
\right ]_+ 
\right \|_2 + 2 R\|C\Tilde{\mathbf{x}}^N - C\hat{\mathbf{x}}^N \|_2  \notag \\
& \leq & 2 R
\left \|
\left [C \hat{\mathbf{x}}^N - \mathbf{b}
\right ]_+ 
\right \|_2 +  2 R\sigma_x \sqrt{\frac{2 \lambda_{max}\left( C^{T}C \right) }{N}} 
 \left (1 + \sqrt{3 \ln \frac{1}{\delta}}
 \right ).
\end{eqnarray}
В силу липшицевости функции $U$ получаем 
\begin{eqnarray*}
|U(\Tilde{\mathbf{x}}^N) - U(\hat{\mathbf{x}}^N) |  \leq M_{U} \|\Tilde{\mathbf{x}}^N - \hat{\mathbf{x}}^N \|_2 \leq M_{U} \sigma_x \sqrt{\frac{2}{N}} 
 \left (1 + \sqrt{3 \ln \frac{1}{\delta}}
 \right ).
\end{eqnarray*}
Тогда
\begin{eqnarray}
\label{part_3}
U(\hat{\mathbf{x}}^N) = U(\Tilde{\mathbf{x}}^N) + \left(U(\hat{\mathbf{x}}^N) - U(\Tilde{\mathbf{x}}^N) \right) \geq U(\Tilde{\mathbf{x}}^N) - M_{U} \sigma_x \sqrt{\frac{2}{N}} 
 \left (1 + \sqrt{3 \ln \frac{1}{\delta}}
 \right ).
\end{eqnarray}
Подставляя~\eqref{part_2} и \eqref{part_3} в \eqref{part_1}, получаем\ev{,} что с вероятность\ev{ю} $1-4\delta$ выполняется 
 \begin{eqnarray*}
 \varphi(\boldsymbol{\hat{\lambda}}^N) 
 & - & U(\Tilde{\mathbf{x}}^N)  + 
2 R
\left \|
\left [C \Tilde{\mathbf{x}}^N - \mathbf{b}
\right ]_+ 
\right \|_2   \le    C_1\dfrac{\sigma\sqrt{ g(N)J} R ^ 2}{\sqrt{N}} 
+ \frac{2 R^2}{\beta N} +
\frac{\beta M^2}{2}  \notag \\ & + &    \frac{ \sqrt{2} \left (1 + \sqrt{3 \ln \frac{1}{\delta}} \right )}{\sqrt{N}}  \left( M_{U} \sigma_x + 2R\left(\sigma + \sigma_x \sqrt{\lambda_{max}\left( C^{T}C \right)} \right) \right). \quad \blacksquare
 \end{eqnarray*}
%~$\blacksquare$

\subsection{Доказательство теоремы~\ref{th_ellipsoid}}
	    
	    Так как $\|\nabla \varphi(\boldsymbol{\lambda})\|_2 \leq M$
	        \ev{ для любых } $\boldsymbol{\lambda} \in \Lambda_{2R}$ \ev{(см.~\eqref{eq_gradM})}, то справедлива следующая оценка
	    $$
	    \sup_{\boldsymbol{\lambda}^1, \, \boldsymbol{\lambda}^2 \, \in \, \Lambda_{2R}} \langle \nabla \varphi(\boldsymbol{\lambda}^1), \, \boldsymbol{\lambda}^2 - \boldsymbol{\lambda}^1 \rangle \leq M \cdot 4R.
	    $$
Из Теоремы 4.1 \cite{nemirovski2010accuracy} получаем, что:
	   % $$
	   % \max_{\boldsymbol{\lambda} \in \Lambda_R} \sum_{t=1}^T \frac{1}{T} \langle \nabla \varphi(\boldsymbol{\lambda}_t), \boldsymbol{\lambda}_t - \boldsymbol{\lambda} \rangle \leq \underbrace{32 \cdot 4 M R \exp \left\{ -\frac{T}{2 n (n+1)} \right\}}_{\varepsilon_T},
	   % $$
	   $$
	    \max_{\boldsymbol{\lambda} \, \in \, \Lambda_{2R}} \sum_{t=1}^N \xi^t \langle \nabla \varphi(\boldsymbol{\lambda}^t), \, \boldsymbol{\lambda}^t - \boldsymbol{\lambda} \rangle \leq \varepsilon_N,
	    $$
где \ai{$\varepsilon_N= 32 \cdot 4 M R \exp \left\{ -\frac{N}{2 m (m+1)} \right\}$.}
Тогда 
\begin{equation*}
    \forall \, \boldsymbol{\lambda} \, \in \, \Lambda_{2R} \, \, \, \, \, \, \,\, \sum_{t \,  \in \, I_{N}} \xi^t \langle \nabla \varphi(\boldsymbol{\lambda}^t), \, \boldsymbol{\lambda}^t - \boldsymbol{\lambda} \rangle \leq \sum_{t=1}^N \xi^t \langle \nabla \varphi(\boldsymbol{\lambda}^t), \, \boldsymbol{\lambda}^t - \boldsymbol{\lambda} \rangle \leq \varepsilon_N.
\end{equation*}
%\pd{Что такое $\varepsilon_N$?}
	   % $$
	   % \sum_{t=1}^T \frac{1}{T} \langle \mathbf{b} - C \mathbf{x}_t, \boldsymbol{\lambda}_t \rangle + \max_{\boldsymbol{\lambda} \in \Lambda_R} \left\langle -\sum_{t = 1}^T \frac{1}{T} (\mathbf{b} - C \mathbf{x}_t), \boldsymbol{\lambda} \right\rangle \leq \varepsilon_T
	   % $$
	   % $$
	   % \Rightarrow 2R \|[C \hat{\mathbf{x}} - \mathbf{b}]_{+}\|_{2} + \sum_{t=1}^T \frac{1}{T} \langle \mathbf{b} - C \mathbf{x}_t, \boldsymbol{\lambda}_t \rangle \leq \varepsilon_T.\qquad (*) 
	   % $$
Отсюда получаем, что верна следующая оценка
	   $$
	    \sum_{t \, \in \, I_{N}} \xi^t \langle \mathbf{b} - C \mathbf{x}^t, \, \boldsymbol{\lambda}^t \rangle + \max_{\boldsymbol{\lambda} \, \in \, \Lambda_R} \left\langle -\sum_{t \, \in \, I_{N}} \xi^t (\mathbf{b} - C \mathbf{x}^t), \, \boldsymbol{\lambda} \right\rangle \leq \varepsilon_N,
	    $$
которую можно переписать в следующем виде
\begin{equation}
\label{eq:est_ellips}
      \sum_{t \, \in \, I_{N}} \xi^t \langle \mathbf{b} - C \mathbf{x}^t, \, \boldsymbol{\lambda}^t \rangle \leq \varepsilon_N - 2R \left \|[C \hat{\mathbf{x}}^N - \mathbf{b}]_{+} \right \|_{2}.
\end{equation}
Далее, \ev{в силу} \eqref{eq_xi_argmax}, для каждого $\mathbf{x} \geq 0$ \ev{и $t \, \in \, I_{N}$} выполнено
	    $$
	    U(\mathbf{x}^t(\boldsymbol{\lambda}^t)) - \langle C \mathbf{x}^t(\boldsymbol{\lambda}^t) - \mathbf{b}, \, \boldsymbol{\lambda}^t \rangle \geq U(\mathbf{x}) - \langle C \mathbf{x} - \mathbf{b}, \, \boldsymbol{\lambda}^t \rangle.
	    $$
Умножая $t$-ое неравенство на $\xi^t$, суммируя по всем индексам из $I_{N}$ и учитывая, что $\sum\limits_{t \, \in \, I_{N}} \xi^t U(\mathbf{x}^t) \leq U(\hat{\mathbf{x}}^{N})$ в силу вогнутости функций $u_k(x_k)$, $k = 1, \, \ldots, \, N$, получаем
	   % $$
	   % U(\mathbf{x}) - U(\hat{\mathbf{x}}) + \langle \mathbf{b} - C \mathbf{x}, \hat{\boldsymbol{\lambda}} \rangle \leq \sum_{t=1}^T \frac{1}{T} \langle \mathbf{b} - C \mathbf{x}_t, \boldsymbol{\lambda}_t \rangle,
	   % $$
	   $$
	    U(\mathbf{x}) - U(\hat{\mathbf{x}}^N) + \langle \mathbf{b} - C \mathbf{x}, \, \hat{\boldsymbol{\lambda}}^N \rangle \leq \sum_{t \in I_{N}} \xi^t \langle \mathbf{b} - C \mathbf{x}^t, \, \boldsymbol{\lambda}^t \rangle,
	    $$
 где $\hat{\boldsymbol{\lambda}}^N = \sum\limits_{t \, \in \, I_{N}} \xi^t \boldsymbol{\lambda}^t$. Используя оценку~\eqref{eq:est_ellips}, получаем, что 
	    \begin{equation} \label{th_pr}
	    2R \left \|[C \hat{\mathbf{x}}^N - \mathbf{b}]_{+} \right \|_{2} + U(\mathbf{x}^{*}) - U(\hat{\mathbf{x}}^N) + \langle \mathbf{b} - C \mathbf{x}^{*}, \, \hat{\boldsymbol{\lambda}}^N \rangle \leq \varepsilon_N.
	    \end{equation}
Поскольку $\hat{\boldsymbol{\lambda}}^N \in \Lambda_{2R}$, и\ev{,} следовательно\ev{,} $\hat{\boldsymbol{\lambda}}^N \geq 0$, откуда $\langle \mathbf{b} - C \mathbf{x}^{*}, \hat{\boldsymbol{\lambda}}^N \rangle \geq 0$, 
%мы приходим к неравенству
\ev{из~\eqref{eq:est_ellips} следует, что}
$U(\mathbf{x}^{*}) - U(\hat{\mathbf{x}}^N) \leq \varepsilon_N$. 
Далее, так как для всех $\mathbf{x} \geq 0$, в силу определения $\boldsymbol{\lambda}^{*}$,
\ev{выполняется} $U(\mathbf{x}^{*}) \geq U(\mathbf{x}) - \langle \boldsymbol{\lambda}^{*}, \, C \mathbf{x} - \mathbf{b} \rangle$, получаем, что 
\begin{align*}
U(\hat{\mathbf{x}}^N)& \leq U(\mathbf{x}^{*}) - \langle \boldsymbol{\lambda}^{*}, \, \mathbf{b} - C \hat{\mathbf{x}}^N \rangle \leq  U(\mathbf{x}^{*}) - \min_{\boldsymbol{\lambda} \, \in
\, \lambda_{R}} \left\{\langle \boldsymbol{\lambda}, \, \mathbf{b} - C \hat{\mathbf{x}}^N \rangle \right\}=\\
&  U(\mathbf{x}^{*}) + \max_{\boldsymbol{\lambda} \, \in \, \lambda_{R}} \left\{\langle \boldsymbol{\lambda}, \, C \hat{\mathbf{x}}^N - \mathbf{b} \rangle \right\} \leq U(\mathbf{x}^{*}) + R \left \|[C \hat{\mathbf{x}}^N - \mathbf{b}]_{+} \right \|_{2}.
\end{align*}
Отсюда вместе с \eqref{th_pr} получаем $\evv{R} \|[C \hat{\mathbf{x}}^N - \mathbf{b}]_{+}\|_2 \leq \varepsilon_N$. Оценка~\eqref{th_saga} на количество итераций метода  следует из следующей выкладки:
$$
\varepsilon_N = 32 \cdot 4 M R \exp \left\{- \frac{N}{2m(m+1)}\right\} \leq \varepsilon \Rightarrow -\frac{N}{2m(m+1)} \leq \ln \left(\frac{\varepsilon}{32\cdot 4 M R}\right) \Rightarrow
$$
$$
\Rightarrow N \geq 2m(m+1) \ln \left(\frac{32 \cdot 4 M R}{\varepsilon}\right). \quad ~\blacksquare
$$
